# Supplementary material for: Energy-Efficient Joint Offloading and Resource Allocation for Deadline-Constrained Tasks in Multi-Access Edge Computing
Source: arXiv:2509.11162 source file (2025-09-14)
Supplement: Supplementary file 1 [file appendix.pdf]

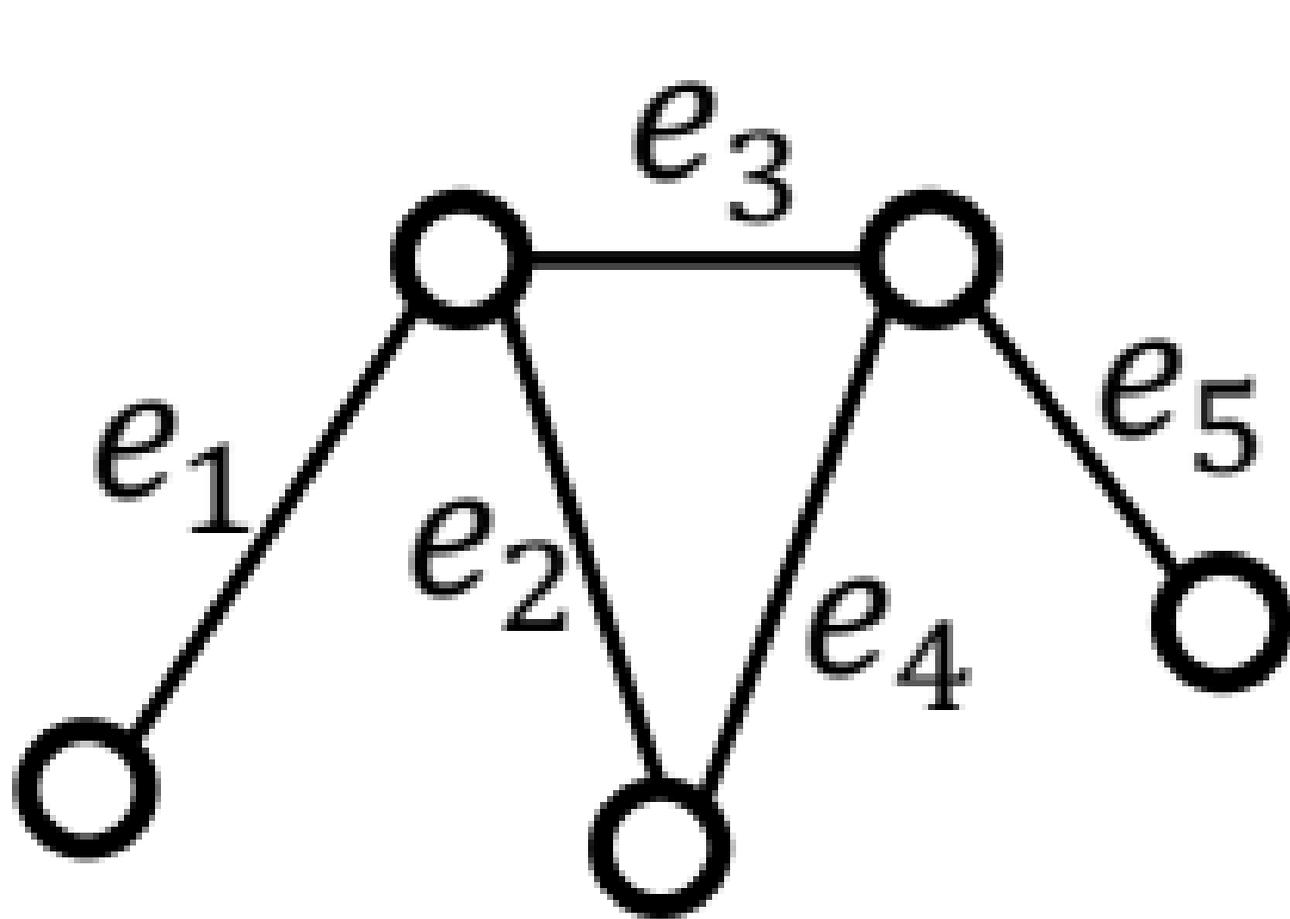

fractional matching  $m$

$$m_{e_1} = 0.7, m_{e_2} = 0.3,$$

$$m_{e_3} = 0, m_{e_4} = 0.3,$$

$$m_{e_5} = 0.7$$

(integral) matching  $m$

$$m_{e_1} = 1, m_{e_2} = 0,$$

$$m_{e_3} = 0, m_{e_4} = 1,$$

$$m_{e_5} = 0$$

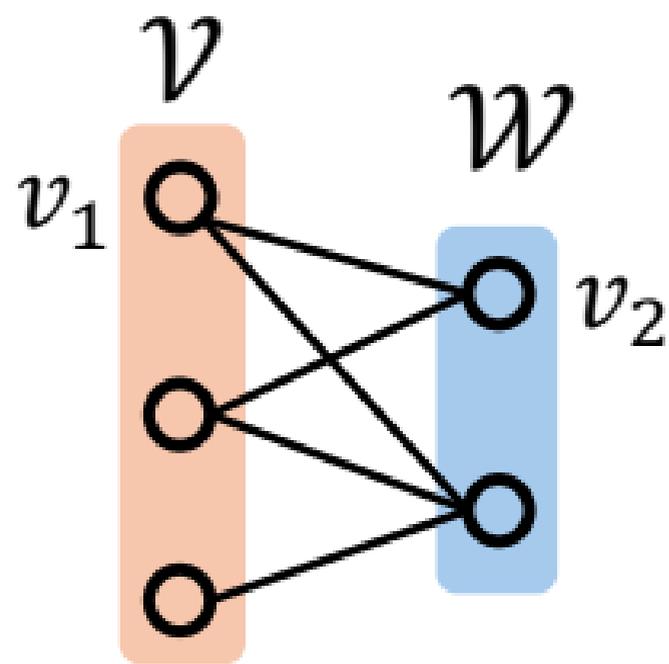

e.g.,  $e_1 = (v_1, v_2)$

bipartite graph

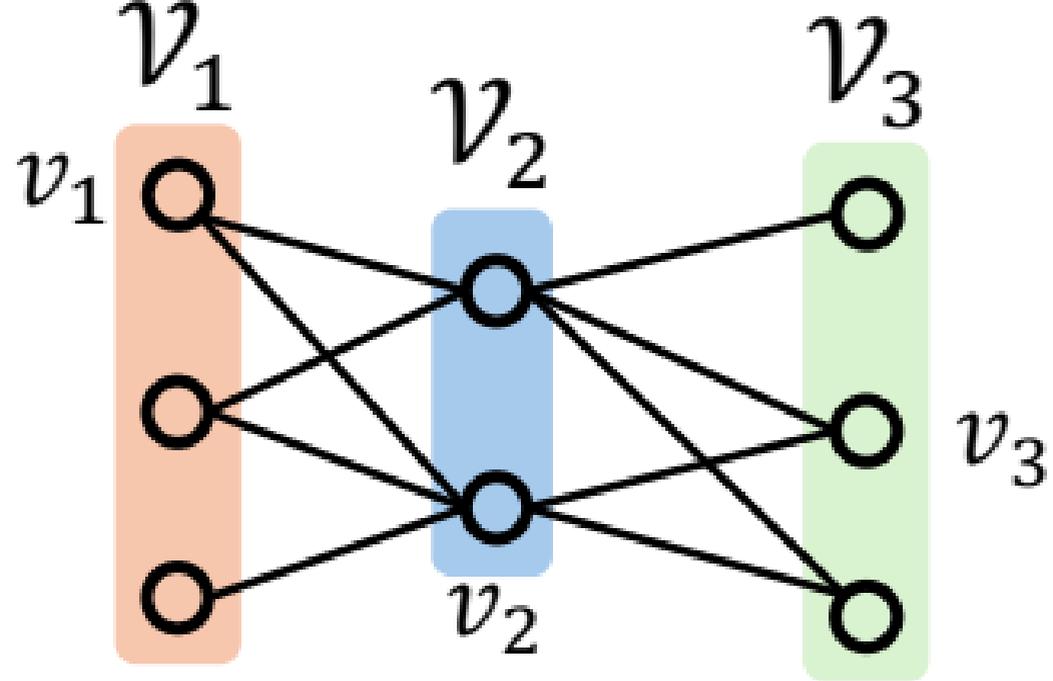

e.g.,  $e_1 = (v_1, v_2, v_3)$

tripartite graph
